# Supplementary material for: DRIFT: Deep Reinforcement Learning for Functional Software Testing
Source: arXiv:2007.08220 source file (2020-07-16)
Supplement: Supplementary file 1 [file appendix.tex]

\appendix
\section{Additional Results}
